# Supplementary material for: Measurement of Spin Correlations in $t\bar{t}$ Events from $pp$ Collisions at $\sqrt{s}$ = 7 TeV in the Lepton + Jets Final State with the ATLAS Detector
Source: arXiv:1410.1791 source file (2014-10-05)
Supplement: Supplementary file 1 [file lepflavcons.tex]

\section{Consistency of Results Across Lepton Flavours}
\label{sec:app_lepflavcons}

For consistency across different lepton flavours a further set of plots is provided.  For each analyser, jet and b-tag multiplicity bin, the SM prediction of \dphi\ is plotted for the \ejet\ (red lines) and the \mujet\ (blue lines) channel as well as the according data. Ratios of data (solid) to prediction (dashed) are also shown as well as the ratio of these two ratios (green). These plots are provided for the \dQ\ in Figure \ref{fig:lepflavorcons_dQ} and the for \bQ\ in Figure \ref{fig:lepflavcons_bQ}.

\begin{figure}[htbp]
\begin{center}
\includegraphics[width=0.45\textwidth]{images/appendix/flavorcomp/4jex_1bex.eps} 
\includegraphics[width=0.45\textwidth]{images/appendix/flavorcomp/4jex_2bin.eps} \\
\includegraphics[width=0.45\textwidth]{images/appendix/flavorcomp/5jin_1bex.eps} 
\includegraphics[width=0.45\textwidth]{images/appendix/flavorcomp/5jin_2bin.eps} 
\end{center}
\caption{The SM prediction (dashed) of $\Delta \phi(l,d)$ for the \ejet\ (red lines) and the \mujet\ (blue lines) channel as well as the according data (solid). Ratios of data to prediction are also shown as well as the ratio of these two ratios (green). 
}
\label{fig:lepflavorcons_dQ}
\end{figure} 

\begin{figure}[htbp]
\begin{center}
\includegraphics[width=0.45\textwidth]{images/appendix/flavorcomp/4jex_1bex_bQ.eps} 
\includegraphics[width=0.45\textwidth]{images/appendix/flavorcomp/4jex_2bin_bQ.eps} \\
\includegraphics[width=0.45\textwidth]{images/appendix/flavorcomp/5jin_1bex_bQ.eps} 
\includegraphics[width=0.45\textwidth]{images/appendix/flavorcomp/5jin_2bin_bQ.eps} 
\end{center}
\caption{The SM prediction (dashed) of $\Delta \phi(l,b)$ for the \ejet\ (red lines) and the \mujet\ (blue lines) channel as well as the according data (solid). Ratios of data to prediction are also shown as well as the ratio of these two ratios (green). 
}
\label{fig:lepflavcons_bQ}
\end{figure}
